# Supplementary material for: Predicting Long Term Sequential Policy Value Using Softer Surrogates
Source: arXiv:2412.20638 source file (2025-02-03)
Supplement: Supplementary file 1 [file supplement_synthetic.tex]

We design a low signal-to-ratio environment with surrogates to evaluate the robustness of Short Long Regression estimators to model mis-specification of a density ratio estimator and a regressor. Similarly as before, our goal is to estimate the long-term returns under a new target policy $\pi_2$ only using short-term state trajectories observed under $\pi_2$ and a historical dataset of short-term state trajectories and their corresponding long-term returns under $\pi_b$. First we introduce the synthetic domain details: states, transitions, returns, and surrogacy.

\paragraph{Domain}Initial states $s_0$ are evenly spaced between [0, 1.5] with additive $N(0, 0.1)$ noise. Under $\pi_b$, transitions to the next state are as follows:

\[
s_1 =
\begin{cases} 
s_0 & \text{w.p 0.5} \\
(-0.6 + 0.1 * U[0,1)) * s_0 & \text{w.p 0.45} \\
1.5 & \text{otherwise}
\end{cases}
\] with additive noise from $N(0, 0.1)$.
Under $\pi_2$, the next state is determined deterministically as:
\[
s_1 =
\begin{cases} 
1.5 & \text{if $s_0 < 1.25$} \\
0 & \text{otherwise}
\end{cases}
\]
plus additive noise from $N(0, 0.1)$. The true long-term return $V^{\pi_b} = V^{\pi_2} = f(s_0, s_1)$ with a quadratic function $f(s_0, s_1) = 5 s_0 + s_1 + s_1^2$. The observed return under $\pi_b$ $V^{\pi_b}_{MC} = V^{\pi_b} + N(0, \omega)$ where $\omega$ determines the amount of noise in the delayed returns (i.e., the higher the $\omega$, the more reliable the regression estimates are compared to the Monte Carlo estimates, same amount of noise is applied to the returns under $\pi_2$). $|D_b| = 5000$, and $|D_2| = 100$. 

We fit an ordinary least squares regression model using `statsmodel` packages. A correct regressor given $(s_0, s_1)$ is fitted as: $f_\theta(s_0, s_1) = \theta^\top [s_0, s_1, s_1^2]$. The continuous states are discretized into 50 bins (thus making a total of 2500 bins for $(s_0, s_1)$), and the number of occurrences per bin is counted to estimate the density ratio between $p(s_0, s_1|\pi_2, \mathcal M_2)$ and $p(s_0, s_1|\pi_b, \mathcal M_b)$. We report the mean squared error of the true and the estimated rewards of the 100 target trajectories under $\pi_2$: $\sqrt{\frac{1}{|D_{2}|}\sum_{i=1}^{100} (\hat V^{\pi_2}_i - V^{\pi_2}_i)^2}$. The code for Table 1 is available as ``surrogate synthetic.py" and the remaining experiments with ``surrogate.py" using --Ntrain 5000 --Ntarget 100. 

\begin{table}[h]
\centering
\caption{\textbf{We show the mean and standard deviation of Mean-Squared Error (MSE) with 200 datasets where the randomness comes from the stochastic transitions under $\pi_b$ and gaussian noises.}}
% \begin{tabular}{@{}lcc@{}}
% \toprule
%  & \begin{tabular}[c]{@{}l@{}}Large noise \\ ($\omega = 10$)\end{tabular} & \begin{tabular}[c]{@{}c@{}}Small noise \\ ($\omega = 1$)\end{tabular} \\ \midrule
% Short long estimator with unweighted regressor   & \textbf{0.11 (0.15)}    &   \textbf{0.002 (0.002)}  \\
% Monte Carlo full returns estimate   &  103.63 (11.24)   &  0.99 (0.16)   \\ \bottomrule
% \end{tabular}
\begin{tabular}{@{}lcc@{}}
\toprule
 & \begin{tabular}[c]{@{}l@{}}Large noise \\ ($\omega = 10$)\end{tabular} & \begin{tabular}[c]{@{}c@{}}Small noise \\ ($\omega = 1$)\end{tabular} \\ \midrule
Short long estimator with unweighted regressor   & \textbf{0.251 (0.307)}    &   \textbf{0.002 (0.003)}  \\
Monte Carlo full returns estimate   &  98.457 (13.355)   &  0.984 (0.133)   \\ \bottomrule
\end{tabular}
\label{table:synthetic_noise}
\end{table}

As discussed in the main text, Table \ref{table:synthetic_noise} shows that our estimates using the short trajectory data provides give more accurate predictions of $V^{\pi_2}$ than using a Monte Carlo estimates of the full return $V^{\pi_2}_{MC}$. Here the regressor is correctly specified, and the comparison is only between the surrogate-based regression estimates and the noisy Monte Carlo estimates.

\paragraph{Model Mis-specification}Next we consider either regressor or density ratio estimator misspecification. A correct regressor is a quadratic function of $s_0, s_1$: $f(s_0, s_1) = 5 s_0 + s_1 + s_1^2$ as stated above, but we use a mis-specified regressor model, in particular a linear model, $f_{\tilde \theta}(s_0, s_1) = {\tilde \theta}^\top [s_0, s_1]$. Note that this linear model can still capture the distribution under $\pi_2$ since $s_1$ under $\pi_2$ is either 0 or 1.5, but not under $\pi_b$. This is by design to show that even when the regression model is mis-specified, when the density ratio estimates are correct, the target estimates can still be accurate as long as the behavioral data supports the target data distribution. We expect the weighted regressor and the doubly robust estimator to be unaffected but the unweighted regressor to fit the target data poorly.

In order to estimate the density ratios, the continuous states are discretized into 50 bins (thus making a total of 2500 bins for $(s_0, s_1)$), and the number of occurrences per bin is counted under $\pi_2$ and under $\pi_b$. Then to  bias the density ratio estimates, we add a non-zero gaussian noise from N(10, 10) to the denominator representing $p(s_0, s_1|\pi_b, \mathcal M_b)$ in the density ratios between $p(s_0, s_1|\pi_2, \mathcal M_2)$  and $p(s_0, s_1|\pi_b, \mathcal M_b)$. We expect the unweighted Short Long Regression estimator and the doubly robust estimator to be unaffected by the density ratio mis-specification as the regressor model is still correct.

\paragraph{Results}
\begin{table}[h]
\centering
\caption{\textbf{We show the MSE of estimators for synthetic example ($\omega = 1$) when regression model or density ratio model may be mis-specified. Mean and std from 200 datasets where the randomness comes from the stochastic transitions under $\pi_b$ and gaussian noises.}}
% \resizebox{\linewidth}{!}{
% \begin{tabular}{@{}lccc@{}}
% \toprule 
%  & Realizable & Regressor Model Misspecified & Density Ratio Model Misspecified \\ \midrule
%  Short long estimator with unweighted regressor  & 0.98 (0.13)   & \textbf{1.89 (0.23)} & 0.98 (0.13) \\
% Short long regression estimator   & 1.07 (0.17)   & 1.07 (0.17)   & \textbf{1.37 (0.71)}  \\ 
% DR short long estimator & 0.99 (0.13)   &  0.99 (0.13) & 0.99 (0.13) \\ \bottomrule
% \end{tabular}}
\resizebox{\linewidth}{!}{
\begin{tabular}{@{}lccc@{}}
\toprule 
 & Realizable & Regressor Model Misspecified & Density Ratio Model Misspecified \\ \midrule
 Short long estimator with unweighted regressor  & 0.002 (0.003)   & \textbf{0.914 (0.064)} & 0.002 (0.003) \\
Short long regression estimator   & 0.079 (0.085)   & 0.080 (0.068)   & \textbf{0.388 (0.728)}  \\ 
DR short long estimator & 0.008 (0.007)   &  0.008 (0.007) & 0.006 (0.005) \\ \bottomrule
\end{tabular}}
% }
\label{table:synthetic_weighted}
\end{table}

Table \ref{table:synthetic_weighted} compares the performance of the 3 different regressors under different conditions. As expected, the doubly robust method does well in all three cases. The short long estimator with weighted regression continues to perform well when the density model is well specified, when fitting a (misspecified) linear regression model, because $V^{\pi_2}$ can be well fit with a linear function. Note however that this method performs less well when the density ratio model is misspecified, since the incorrect weights impact the learned regression model. Note that we consider the use of a linear regression model as misspecification in this case because because the linear model is only correct for the processes under $\pi_2$ and not for the processes under $\pi_b$, which require a quadratic.

Even when the density ratio estimates are incorrect, unweighted and DR estimates perform well when the regressor is correctly specified. Since the regression model itself is still consistent, as the training data size increases, the effect due to the incorrect density ratio estimates is lessened for the weighted short long horizon regression estimate, as we show in  in Table \ref{table:synthetic_weighted2}. 

Our synthetic experiments demonstrate that the doubly robust estimator is robust to both regressor and density ratio estimator misspecification. The unweighted estimator has a higher error when the regression model is misspecified, and the weighted estimator  has higher error when the density ratio model is misspecified (since this impacts the regression fit due to a limited training sample size).

\begin{table}[h]
\centering
\caption{\textbf{MSE using different training data sizes of the short long regression estimator when the density ratio estimates are misspecified.}}
\begin{tabular}{@{}lc@{}}
\toprule
Training data size &  Error \\ \midrule
500  & 2.123 (7.382) \\
1000  & 0.806 (1.281) \\
% 5000 & 1.37 (0.71) \\
% 10000 & 1.27 (0.43) \\
50000 & 0.259 (0.480) \\
 \bottomrule
\end{tabular}
% \begin{tabular}{@{}lc@{}}
% \toprule
% Training data size &  Error \\ \midrule
% 500  & 3.11 (7.27) \\
% 1000  & 1.80 (1.29) \\
% % 5000 & 1.37 (0.71) \\
% % 10000 & 1.27 (0.43) \\
% 50000 & 1.17 (0.42) \\
%  \bottomrule
% \end{tabular}
\label{table:synthetic_weighted2}
\end{table}
